# Supplementary material for: Radiance-Field Guided Pretraining: Scaling Localization Models with Unlabeled Wireless Signals
Source: arXiv:2512.07309 source file (2026-09-22)
Supplement: Supplementary file 1 [file appendix.tex]

\appendixname

\appendix

\section{Dataset}
\label{appendix:dataset}

\begin{table*}[htbp]
\centering
\begin{threeparttable}
\scriptsize 
\setlength{\tabcolsep}{2pt} 

\vspace{-48pt}
\caption{Summary of wireless datasets}
\label{tab:datasets}
\begin{tabular}{|c|c|c|c|c|c|c|c|c|c|}
\toprule
\rowcolor[HTML]{000000} 
{\color[HTML]{FFFFFF} \textbf{Technology}} & 
{\color[HTML]{FFFFFF} \textbf{Frequency}} &  
{\color[HTML]{FFFFFF} \textbf{Source}} &
{\color[HTML]{FFFFFF} \textbf{Scene}\tnote{*}} & 
{\color[HTML]{FFFFFF} \textbf{RSS/SNR}\tnote{**}} & 
{\color[HTML]{FFFFFF} \textbf{Total}} & 
{\color[HTML]{FFFFFF} \textbf{Den.}\tnote{***}} & 
{\color[HTML]{FFFFFF} \textbf{Station}} & 
{\color[HTML]{FFFFFF} \textbf{Range}} & 
{\color[HTML]{FFFFFF} \textbf{Temperature}} \\ 
%{\color[HTML]{FFFFFF} \textbf{Pretrain}}\\
\rowcolor[HTML]{000000} 
{\color[HTML]{FFFFFF} \textbf{(\#)}} & 
{\color[HTML]{FFFFFF} \textbf{(\#)}} & 
{\color[HTML]{FFFFFF} \textbf{}} & 
{\color[HTML]{FFFFFF} \textbf{(\#)}} & 
{\color[HTML]{FFFFFF} \textbf{(dBm)/(dB)}} & 
{\color[HTML]{FFFFFF} \textbf{(\#)}} & 
{\color[HTML]{FFFFFF} \textbf{(p/m$^3$)}} & 
{\color[HTML]{FFFFFF} \textbf{(\#)}} & 
{\color[HTML]{FFFFFF} \textbf{(m)}} & 
{\color[HTML]{FFFFFF} \textbf{(\textdegree C)}} \\ 
%{\color[HTML]{FFFFFF} \textbf{}} \\
\midrule

\multirow{34}{*}{\rotatebox{90}{RFID}} & \multirow{34}{*}{\rotatebox{90}{920MHz}} & \multirow{34}{*}{Ours}  & P1 & -62.5 & 84,392 & 3,843 & 3 & 5 & 31.2 \\
 & & & P2 & -66.4 & 57,311 & 4,689 & 3 & 10 & 30.3 \\
 & & & P3 & -66.7 & 55,527 & 5,274 & 3 & 15 & 29.9 \\
 & & & P4 & -71.0 & 50,302 & 4,336 & 3 & 25 & 27.2 \\
 & & & P5 & -75.0 & 51,241 & 5,866 & 3 & 30 & 27.4 \\
 & & & P6 & -77.4 & 51,289 & 5,871 & 3 & 35 & 27.7 \\
 & & & P7 & -78.8 & 74,521 & 7,834 & 3 & 40 & 28.1 \\
 & & & P8 & -79.1 & 76,475 & 5,224 & 3 & 50 & 29.0 \\
 & & & P9 & -88.6 & 50,186 & 10,490 & 3 & 55 & 28.7 \\
 & & & P10 & -71.8 & 23,028 & 539 & 3 & 25 & 30.1 \\
 & & & P11 & -78.1 & 38,303 & 1,382 & 3 & 40 & 30.9 \\
 & & & P12 & -68.3 & 18,726 & 6,080 & 3 & 20 & 33.1 \\
 & & & P13 & -67.0 & 40,571 & 2,546 & 3 & 13 & 28.8 \\
 & & & P14 & -66.2 & 160,494 & 38,213 & 3 & 10 & 18.4 \\
 & & & P15 & -65.3 & 78,635 & 27,924 & 2 & 10 & 24.9 \\
 & & & P16 & -63.7 & 30,103 & 10,907 & 2 & 10 & 25.1 \\
 & & & P17 & -65.4 & 32,042 & 5,057 & 2 & 10 & 24.8 \\
 & & & P18 & -65.1 & 48,467 & 22,627 & 3 & 7 & 25.8 \\
 & & & P19 & -61.4 & 10,521 & 4,912 & 3 & 5 & 27.5 \\
 & & & P20 & -61.9 & 6,723 & 2,394 & 3 & 5 & 27.3 \\
 & & & P21 & -61.9 & 8,413 & 1,829 & 3 & 5 & 28.2 \\
 & & & P22 & -63.7 & 8,911 & 1,600 & 3 & 5 & 27.9 \\
 \rowcolor[gray]{0.95} & & &  S1 & -69.4 & 54,518 & 3,787 & 3 & 20 & 29.4 \\
 \rowcolor[gray]{0.95} & & &  S2 & -79.3 & 61,909 & 4,236 & 3 & 45 & 28.3 \\
 \rowcolor[gray]{0.95} & & &  S3 & -76.9 & 21,357 & 702 & 3 & 35 & 30.4 \\
 \rowcolor[gray]{0.95} & & &  S4 & -68.9 & 77,538 & 4,345 & 3 & 13 & 29.2 \\
 \rowcolor[gray]{0.95} & & &  S5 & -64.9 & 26,916 & 8,901 & 2 & 10 & 27.6 \\
 \rowcolor[gray]{0.95} & & &  S6 & -60.2 & 5,291 & 938 & 3 & 5 & 30.1 \\
\hline
\multirow{35}{*}{\rotatebox{90}{BLE}} & \multirow{35}{*}{\rotatebox{90}{2.4GHz}} & \multirow{35}{*}{Ours} 
 & P23 & -72.5 & 8,030 & 138 & 4 & 5 & 26.4 \\
 & & & P24 & -84.5 & 11,123 & 199 & 4 & 5 & 26.4 \\
 & & & P25 & -89.2 & 8,967 & 309 & 4 & 5 & 27.1 \\
 & & & P26 & -62.4 & 8,419 & 1,011 & 4 & 5 & 29.3 \\
 & & & P27 & -61.1 & 8,959 & 1,134 & 4 & 5 & 28.8 \\
 & & & P28 & -64.9 & 8,647 & 1,259 & 4 & 5 & 18.3 \\
 & & & P29 & -71.0 & 15,412 & 1,381 & 4 & 20 & 17.8 \\
 & & & P30 & -69.2 & 18,975 & 1,073 & 4 & 10 & 16.8 \\
 & & & P31 & -72.1 & 41,400 & 411 & 3 & 5 & 33.8 \\
 & & & P32 & -73.0 & 130,200 & 1,211 & 3 & 5 & 33.8 \\
 & & & P33 & -75.0 & 272,400 & 2,862 & 3 & 15 & 32.8 \\
 & & & P34 & -73.0 & 306,000 & 3,371 & 3 & 10 & 32.8 \\
 & & & P35 & -68.1 & 399,600 & 3,678 & 3 & 15 & 31.6 \\
 & & & P36 & -67.4 & 379,800 & 3,745 & 3 & 15 & 31.8 \\
 & & & P37 & -69.2 & 309,600 & 3,534 & 3 & 10 & 31.8 \\
 & & & P38 & -78.7 & 343,800 & 3,438 & 3 & 20 & 33.3 \\
 & & & P39 & -77.4 & 331,800 & 4,424 & 3 & 15 & 32.5 \\
 & & & P40 & -63.9 & 362,100 & 3,219 & 3 & 15 & 26.3 \\
 & & & P41 & -83.9 & 323,700 & 5,179 & 3 & 25 & 27.5 \\
 & & & P42 & -92.9 & 43,200 & 1,728 & 3 & 25 & 26.8 \\
 & & & P43 & -63.6 & 328,800 & 13,152 & 3 & 10 & 26.5 \\
 & & & P44 & -53.2 & 305,400 & 24,432 & 3 & 5 & 26.0 \\
 & & & P45 & -87.9 & 332,400 & 3,324 & 3 & 20 & 36.3 \\
 \rowcolor[gray]{0.95} & & &  S7 & -60.4 & 6,386 & 823 & 4 & 5 & 29.9 \\
 \rowcolor[gray]{0.95} & & &  S8 & -61.7 & 8,375 & 607 & 4 & 5 & 28.0 \\
 \rowcolor[gray]{0.95} & & &  S9 & -60.9 & 11,235 & 1,489 & 4 & 5 & 18.5 \\
 \rowcolor[gray]{0.95} & & &  S10 & -72.1 & 4,779 & 239 & 3 & 10 & 27.8 \\
 \rowcolor[gray]{0.95} & & &  S11 & -79.5 & 5,786 & 116 & 3 & 30 & 28.6 \\
 \rowcolor[gray]{0.95} & & &  S12 & -83.7 & 8,878 & 296 & 3 & 15 & 20.3 \\
\hline
\multirow{26}{*}{\rotatebox{90}{IIoT}} &  & \multirow{26}{*}{\cite{dichasus2021}} & P46 & 4.48 & 41,492 & 69 & 4 & 30 & N/A \\
 & & & P47 & 5.24 & 12,576 & 32 & 4 & 27 & N/A \\
 & & & P48 & 5.65 & 47,227 & 81 & 4 & 29 & N/A \\
 \rowcolor[gray]{0.95} & & &  S13 & 4.83 & 12,584 & 28 & 4 & 28 & N/A \\
 \rowcolor[gray]{0.95} & & &  S14 & 1.95 & 10,814 & 31 & 4 & 57 & N/A \\
 \rowcolor[gray]{0.95} & \multirow{-6}{*}{\rotatebox{90}{3.44GHz}}& &  S15 & 5.64 & 27,814 & 47 & 4 & 29 & N/A \\
\cline{4-10}
 & \multirow{17}{*}{\rotatebox{90}{1.27GHz}} & & P49 & 14.1 & 26,464 & 178 & 4 & 13 & N/A \\
 & & & P50 & 14.5 & 35,640 & 237 & 4 & 13 & N/A \\
 & & & P51 & 14.3 & 12,702 & 139 & 4 & 11 & N/A \\
 & & & P52 & 14.2 & 53,087 & 349 & 4 & 13 & N/A \\
 & & & P53 & 14.2 & 27,510 & 210 & 4 & 13 & N/A \\
 & & & P54 & 15.4 & 22,643 & 151 & 4 & 13 & N/A \\
 & & & P55 & 15.3 & 42,158 & 276 & 4 & 13 & N/A \\
 & & & P56 & 11.1 & 14,330 & 87 & 3 & 19 & N/A \\
 & & & P57 & 11.0 & 9,537 & 60 & 3 & 19 & N/A \\
 \rowcolor[gray]{0.95} & & &  S16 & 15.1 & 18,602 & 127 & 4 & 13 & N/A \\
 \rowcolor[gray]{0.95} & & &  S17 & 11.1 & 9,658 & 60 & 3 & 19 & N/A \\
 \rowcolor[gray]{0.95} & & &  S18 & 11.0 & 14,272 & 86 & 3 & 19 & N/A \\
 \rowcolor[gray]{0.95} & & &  S19 & 8.5 & 6,707 & 14 & 3 & 118 & N/A \\
\hline
\multirow{14}{*}{\rotatebox{90}{WiFi I}} & \multirow{14}{*}{\rotatebox{90}{2.4GHz}} & \multirow{14}{*}{Ours}  & P58 & -58.6 & 11,288 & 123 & 4 & 7 & N/A \\
 & & & P59 & -58.6 & 14,543 & 164 & 4 & 7 & N/A \\
 & & & P60 & -60.0 & 10,579 & 106 & 4 & 7 & N/A \\
 & & & P61 & -60.1 & 5,233 & 58 & 4 & 7 & N/A \\
 & & & P62 & -48.2 & 25,976 & 701 & 3 & 4 & N/A \\
 & & & P63 & -48.3 & 16,286 & 497 & 3 & 4 & N/A \\
 & & & P64 & -48.2 & 6,769 & 278 & 3 & 4 & N/A \\
 & & & P65 & -68.2 & 2,767 & 156 & 3 & 4 & N/A \\
 & & & P66 & -64.3 & 1,246 & 112 & 3 & 4 & N/A \\
 & & & P67 & -65.6 & 1,583 & 134 & 3 & 4 & N/A \\
 \rowcolor[gray]{0.95} & & &  S20 & -60.1 & 8,287 & 76 & 4 & 7 & N/A \\
 \rowcolor[gray]{0.95} & & &  S21 & -48.2 & 23,677 & 656 & 3 & 4 & N/A \\
\hline
\multirow{16}{*}{\rotatebox{90}{WiFi II}} & \multirow{16}{*}{\rotatebox{90}{2.4GHz}} & \multirow{16}{*}{\cite{dataset-espargos-0007,dataset-espargos-0001,dataset-espargos-0005, dataset-espargos-0002}}  & P68 & -47.1 & 92,903 & 9,760 & 4 & 3 & N/A \\
 & & & P69 & -47.1 & 139,427 & 6,847 & 4 & 5 & N/A \\
 & & & P70 & -47.1 & 124,980 & 6,173 & 4 & 5 & N/A \\
 & & & P71 & -47.5 & 85,168 & 3,946 & 4 & 5 & N/A \\
 & & & P72 & -67.0 & 154,394 & 13,752 & 4 & 4 & N/A \\
 & & & P73 & -63.8 & 127,241 & 5,797 & 4 & 5 & N/A \\
 & & & P74 & -58.2 & 89,083 & 13,223 & 4 & 3 & N/A \\
 & & & P75 & -57.9 & 77,527 & 12,299 & 4 & 3 & N/A \\
 \rowcolor[gray]{0.95} & & &  S22 & -47.2 & 62,695 & 3,040 & 4 & 5 & N/A \\
 \rowcolor[gray]{0.95} & & &  S23 & -47.4 & 29,965 & 2,902 & 4 & 3 & N/A \\
 \rowcolor[gray]{0.95} & & &  S24 & -66.1 & 71,136 & 7,923 & 4 & 3 & N/A \\
 \rowcolor[gray]{0.95} & & &  S25 & -58.3 & 50,870 & 9,764 & 4 & 2 & N/A \\
\bottomrule
\end{tabular}
\begin{tablenotes}
			\item[*] P<idx> for pretraining, S<idx> for fine-tuning.
            \item[**] SNR in the WLAN dataset, RSS in others.
            \item[***] The Z-axis can be disregarded in the WLAN and WiFi II datasets, as the variations are minimal.
        \end{tablenotes}
    \end{threeparttable}
\end{table*}

\section{Latent Location Feature}
\label{appendix:pos}
